# Supplementary material for: Index Date Imputation for Survival Analysis in Externally Controlled Trials with Delayed Treatment Initiation
Source: arXiv:2509.14183 source file (2026-11-30)
Supplement: Supplementary file 1 [file FDA_CERSI_Index_Date_Supplementary.pdf]

# Supplementary materials for “Index Date Imputation For Survival Outcomes for Externally Controlled Trials”

Quentin Le Coent<sup>1</sup>, Gary Rosner<sup>1</sup>, Mei-Cheng Wang<sup>2</sup>, and Chen Hu<sup>1,2</sup>

<sup>1</sup>Division of Biostatistics, Oncology Department, Johns Hopkins University

<sup>2</sup>Biostatistic Department, Bloomberg School of Public Health, Johns Hopkins University

## **A: Additional figures**

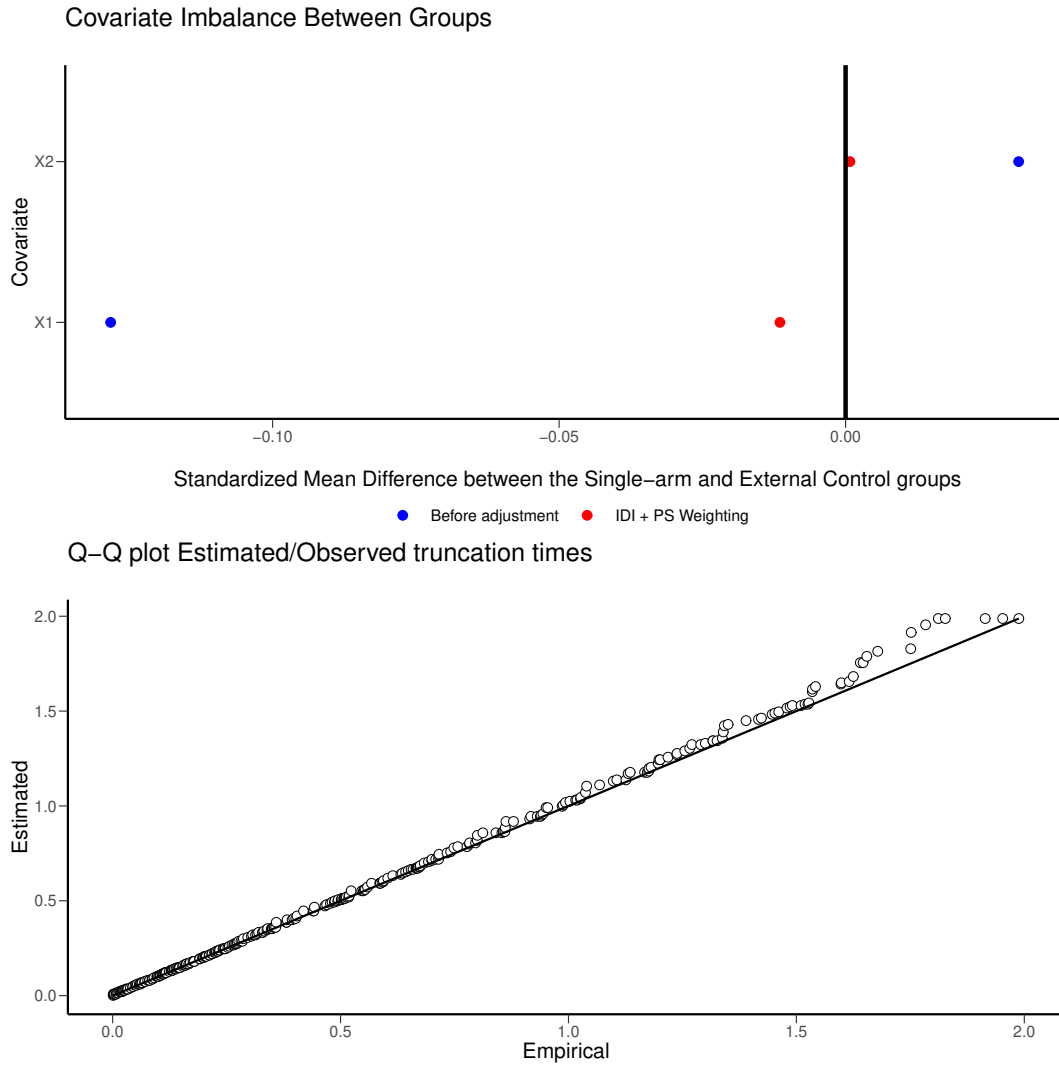

Figure 1: Diagnostic tools. Top figure: covariate imbalance between the single-arm and external control groups before/after adjustment. Bottom figure: Q-Q plot comparing the observed index time distribution in the single-arm with the estimated distribution. Illustration based on a simulated dataset.

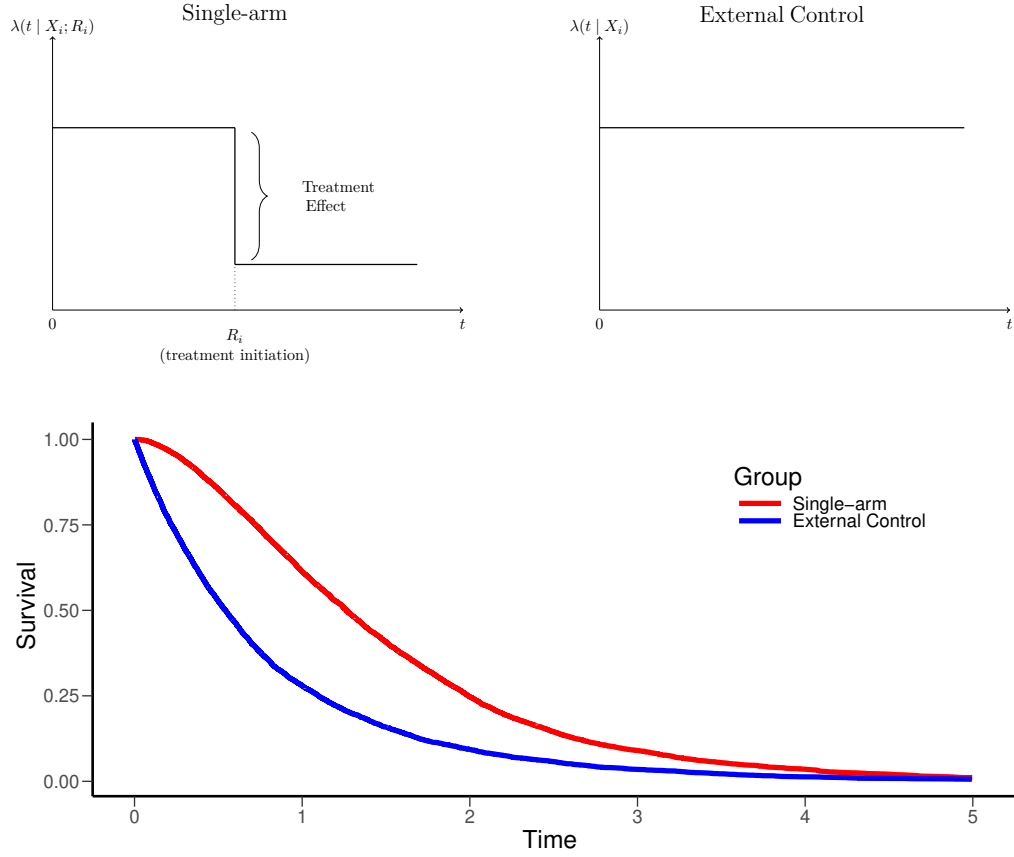

Figure 2: Survival distribution for the simulations study. Top figure: Conditional hazard-function given the covariates  $X_i$  and truncation time  $R_i$  for a single-arm patient (left) and conditional hazard-function given the covariates  $X_i$  for an external-control patient. Bottom figure: Marginal survival functions of the single-arm and external control groups without adjustment for truncation or confounding when  $\alpha = 0$  (no treatment effect).
